# Supplementary material for: Assessing the Impact of Attention and Self-Attention Mechanisms on the Classification of Skin Lesions
Source: arXiv:2112.12748 source file (2021-12-23)
Supplement: Supplementary file 1 [file appendix.tex]

\begin{appendices}

\section{GradCAM and GradCAM++}
One of the objectives throughout this thesis was to verify the reasoning of models with and without attention. Therefore, the GradCAM and GradCAM++ \cite{gradcam} techniques were used to demonstrate the model reasoning through the attention maps. The implementation of  GradCAM and GradCAM++ is inspired by the work of the authors of TA \cite{ta}. In the following images, the left column is the input image, the middle column is the result from GradCAM, and the column to the right is the GradCAM++. The attention maps were obtained for all the studied datasets and every corresponding class. So that the attention maps were more detailed, they were generated with the dataset images of their original size.

In \Cref{fig:akiec,fig:bcc,fig:bkl,fig:df,fig:mel,fig:nv,fig:vasc}, the attention maps for all the seven classes on the HAM10000 dataset are presented. Besides being applied to the competition test set, the trained models were also tested on Grad-CAM and Grad-CAM++. The images come from the validation set. However, they were not randomly sampled. It made more sense to have pictures where at least one of the models would get the prediction right to compare. Other than that, the images are chosen randomly. The architecture tested is the ResNet-50 without pretraining. The attention mechanisms start to look at more specific regions of the image, and they seem to remove the noise from the photos with more ease.

\begin{figure}[H]
\centering
\includegraphics{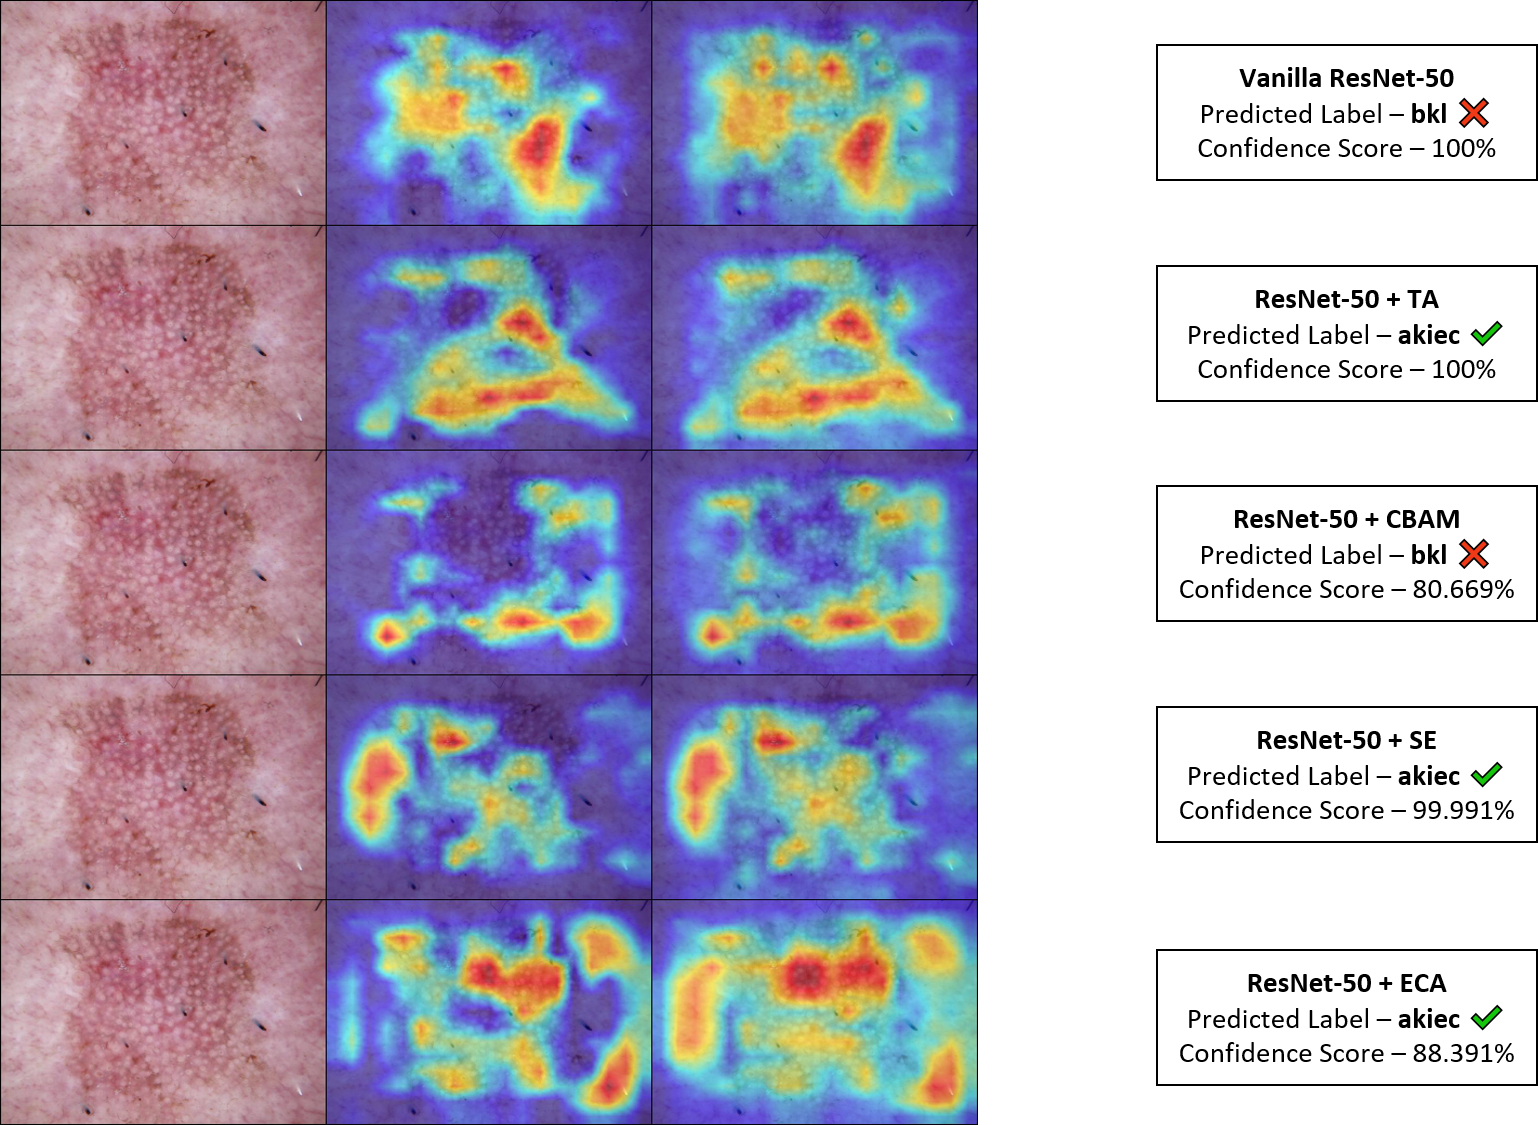}
\caption{Visualization of GradCAM and GradCAM++ respectively in a random example of the validation set in the AKIEC class.}
\label{fig:akiec}
\end{figure}

\begin{figure}[H]
\centering
\includegraphics{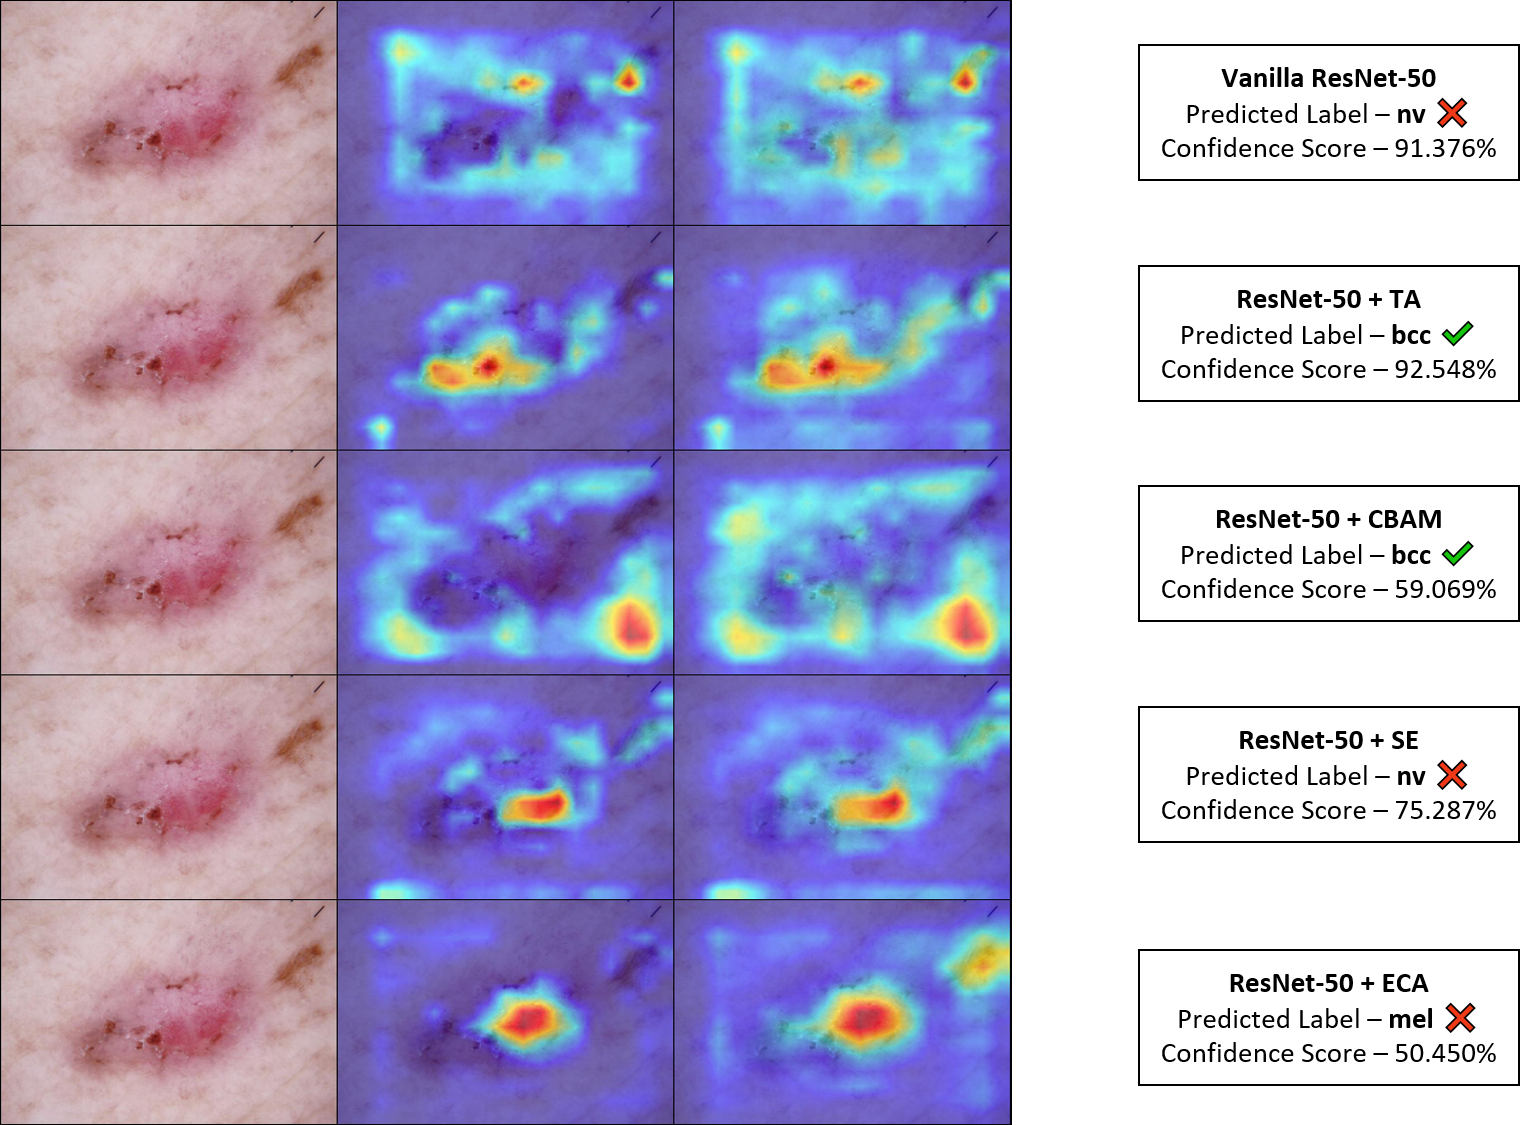}
\caption{Visualization of GradCAM and GradCAM++ respectively in a random example of the validation set in the BCC class.}
\label{fig:bcc}
\end{figure}

\begin{figure}[H]
\centering
\includegraphics{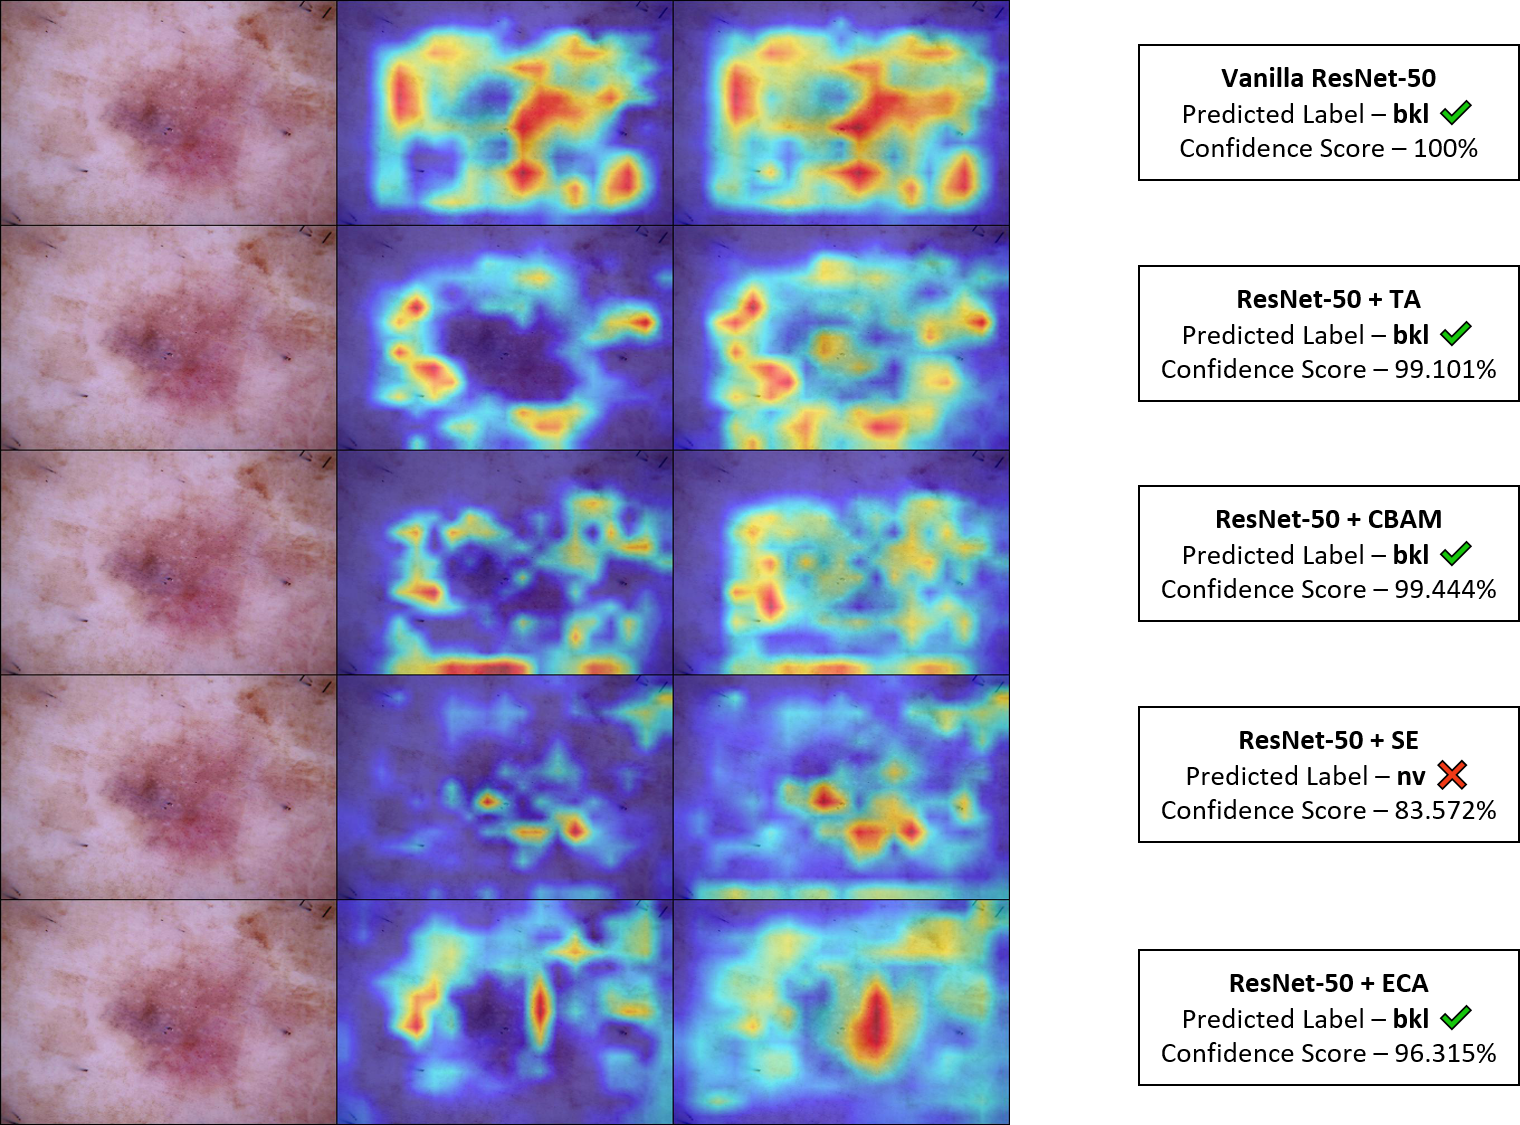}
\caption{Visualization of GradCAM and GradCAM++ respectively of the validation set in the BKL class.}
\label{fig:bkl}
\end{figure}

\begin{figure}[H]
\centering
\includegraphics{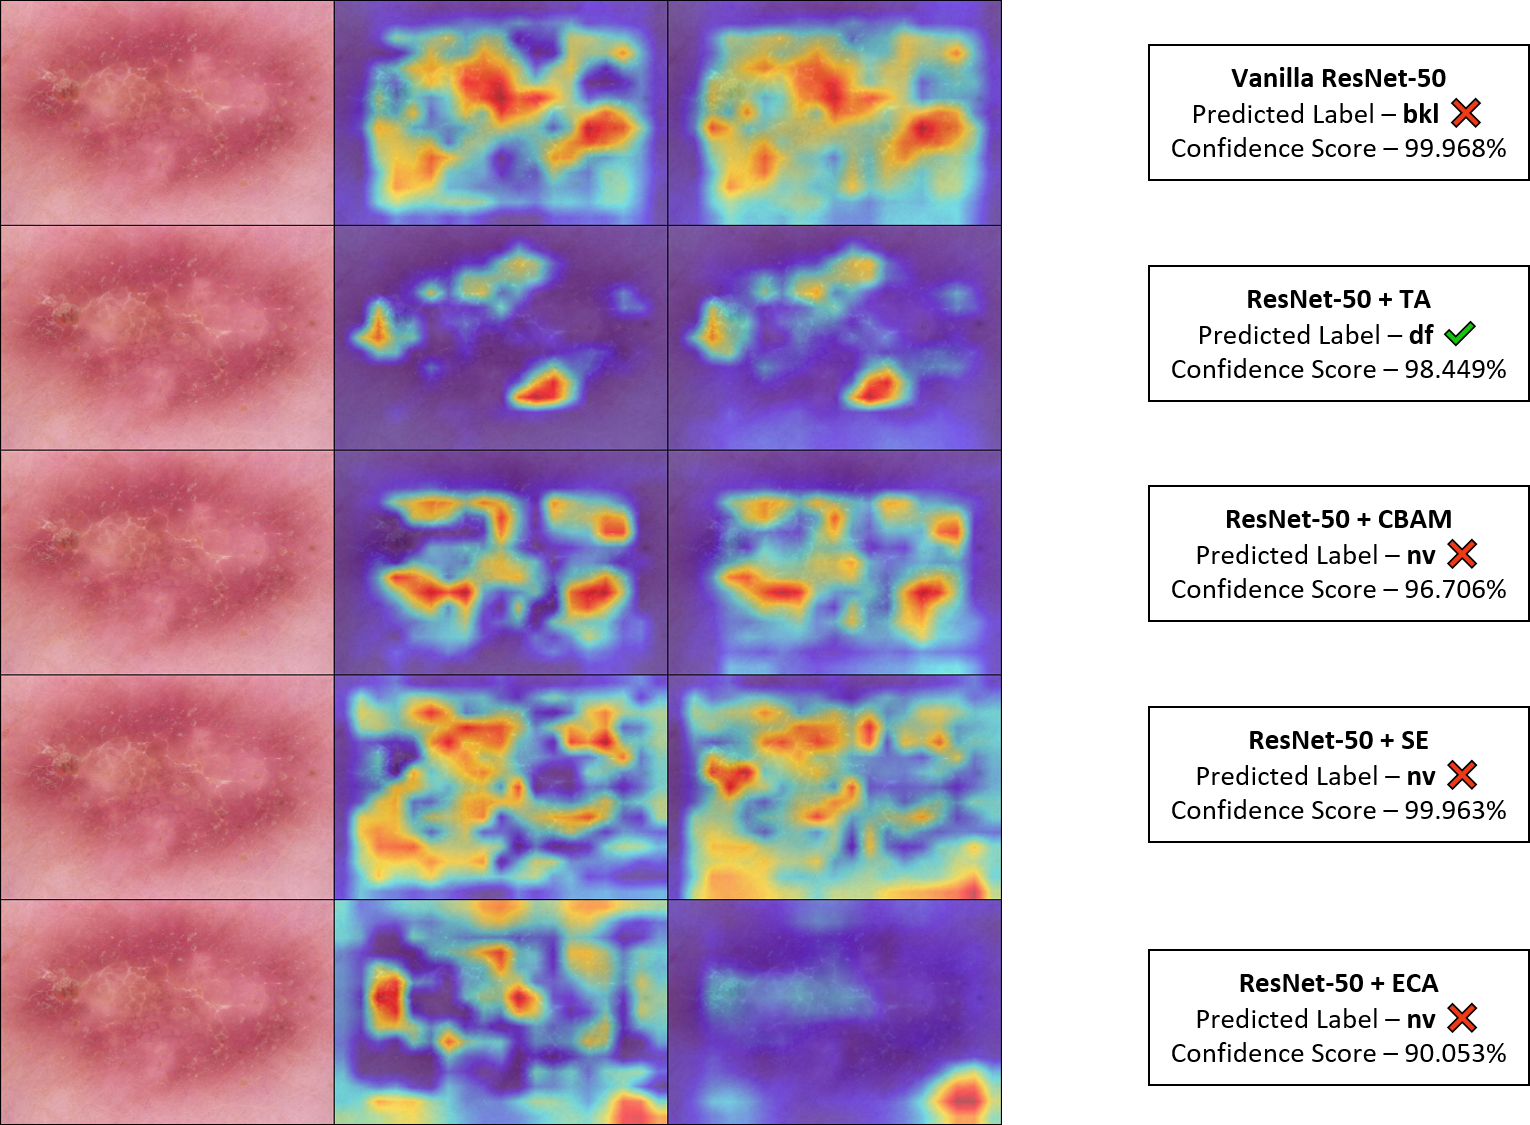}
\caption{Visualization of GradCAM and GradCAM++ respectively of the validation set in the DF class.}
\label{fig:df}
\end{figure}

\begin{figure}[H]
\centering
\includegraphics{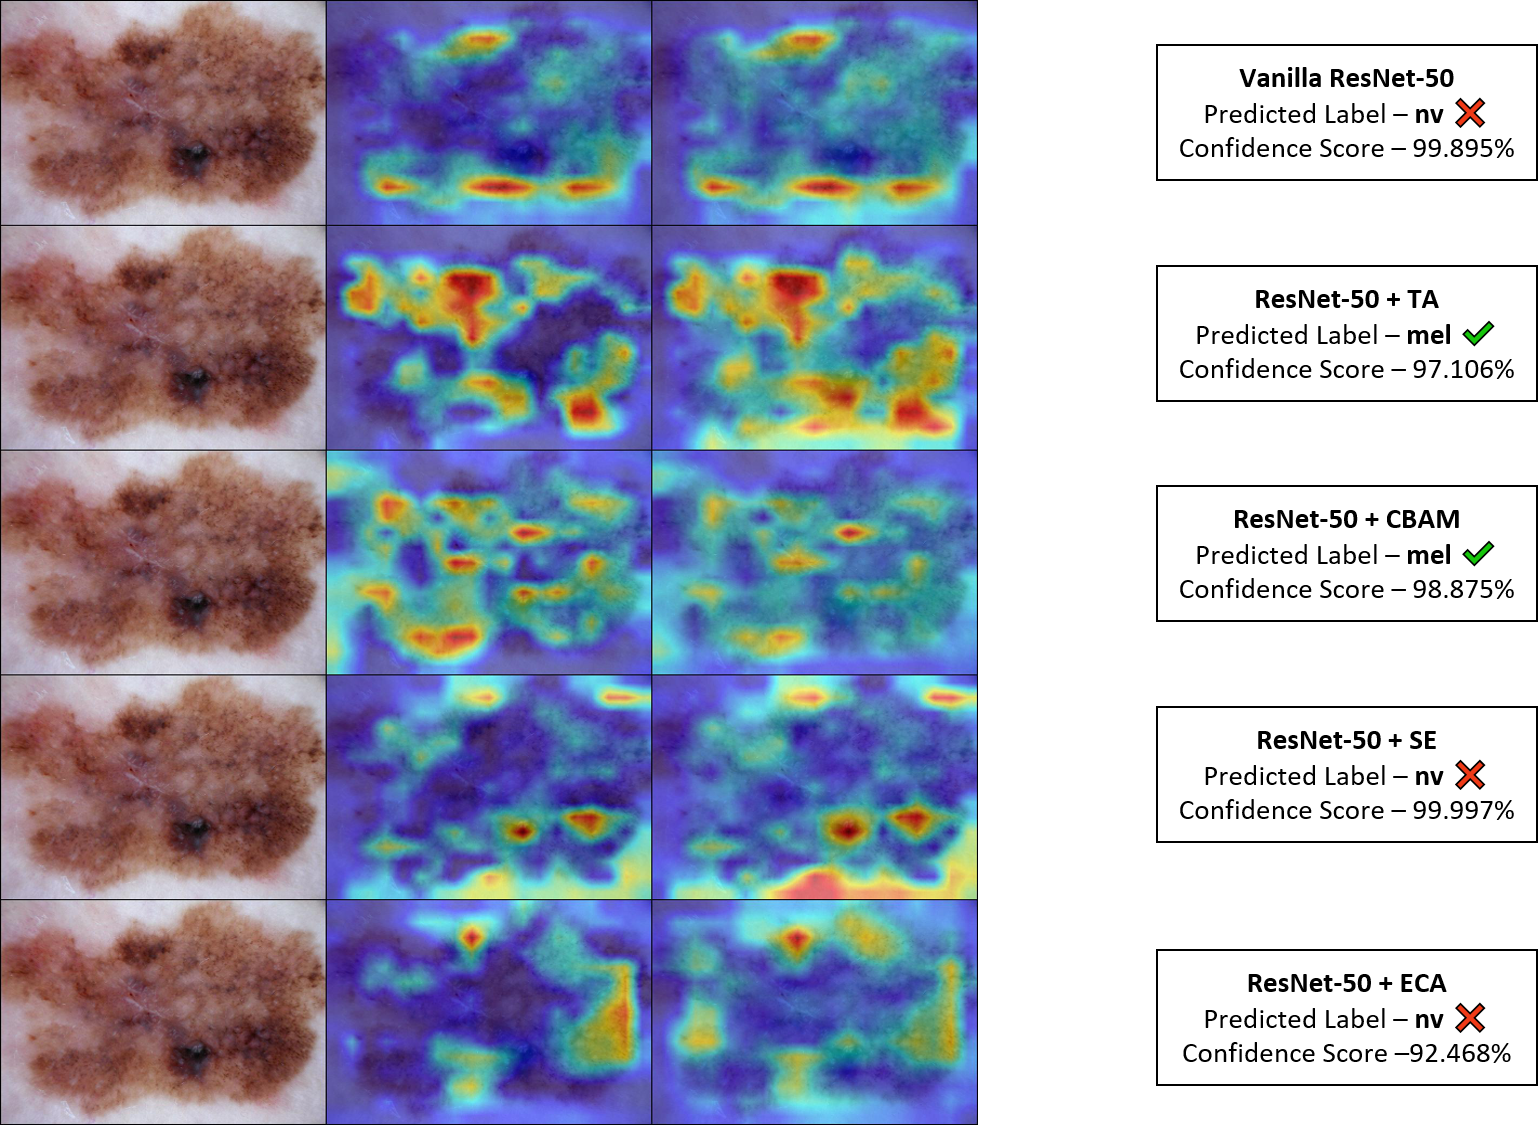}
\caption{Visualization of GradCAM and GradCAM++ respectively of the validation set in the MEL class.}
\label{fig:mel}
\end{figure}

\begin{figure}[H]
\centering
\includegraphics{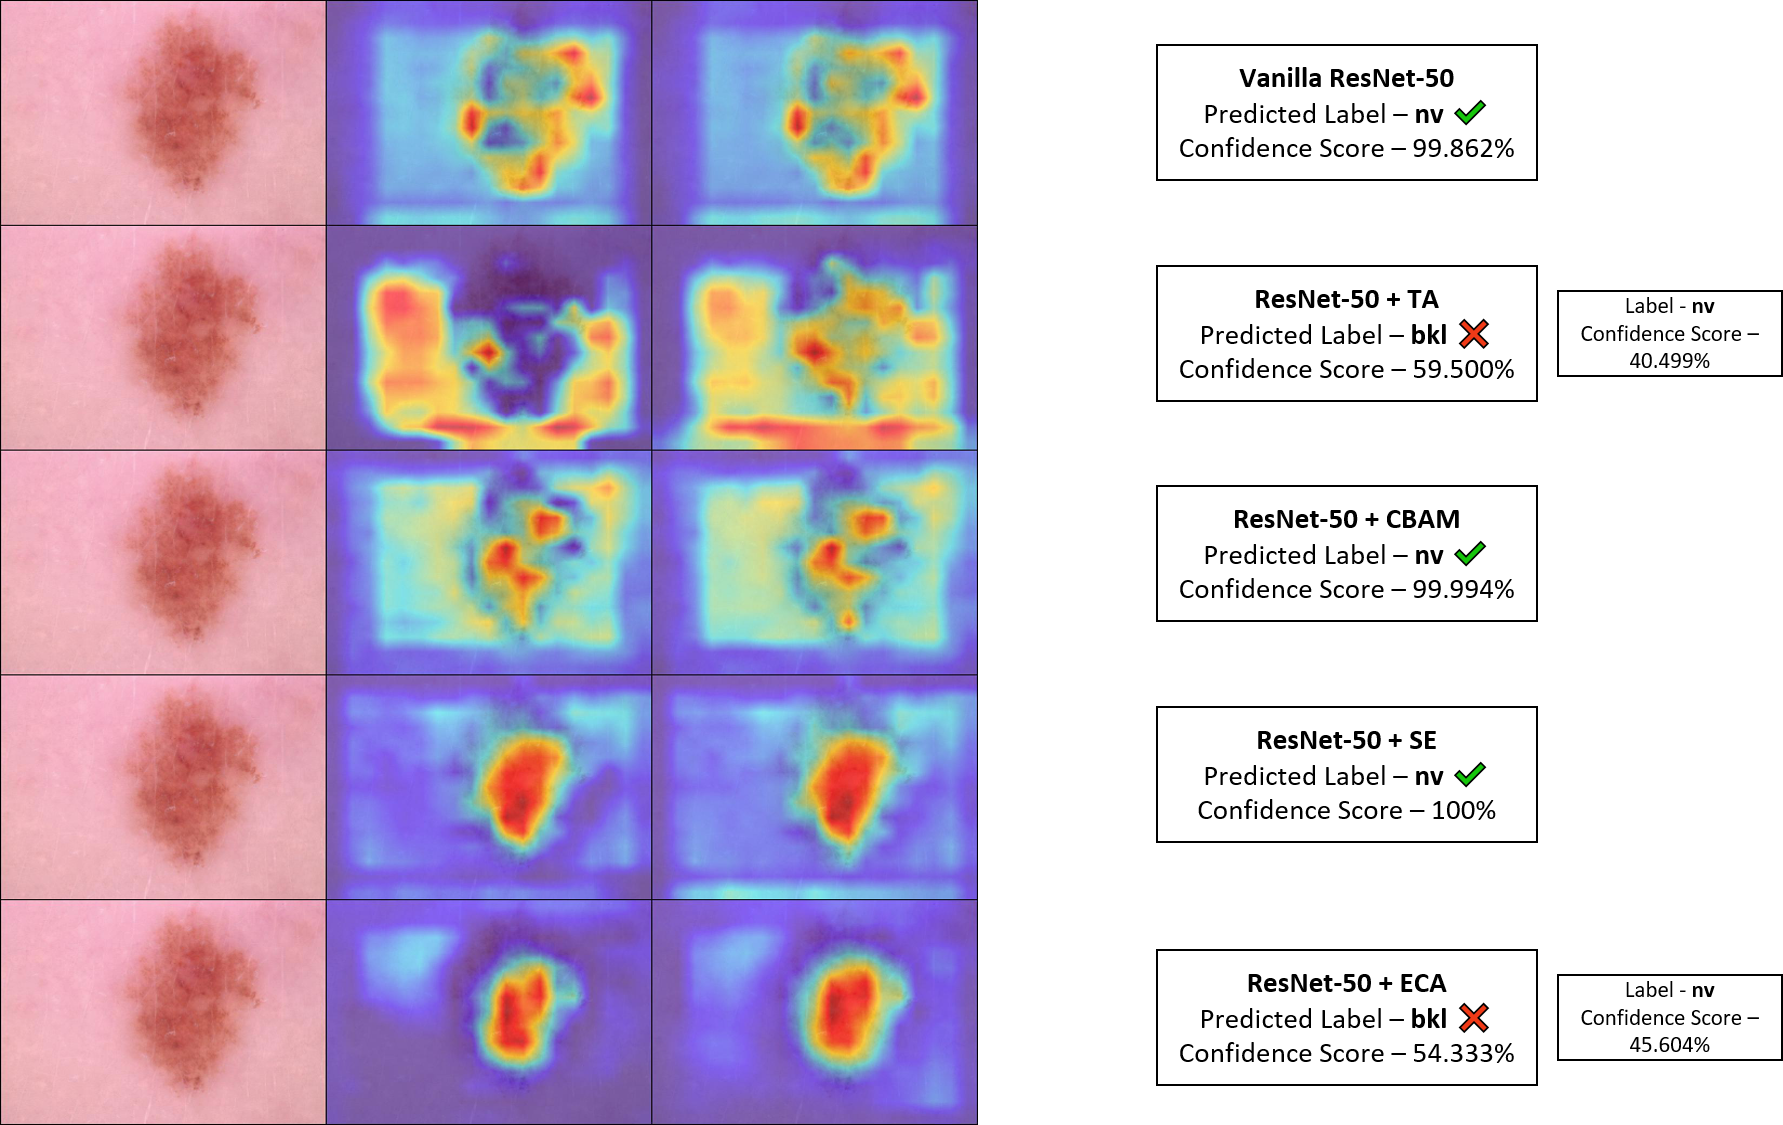}
\caption{Visualization of GradCAM and GradCAM++ respectively of the validation set in the NV class.}
\label{fig:nv}
\end{figure}

\begin{figure}[H]
\centering
\includegraphics{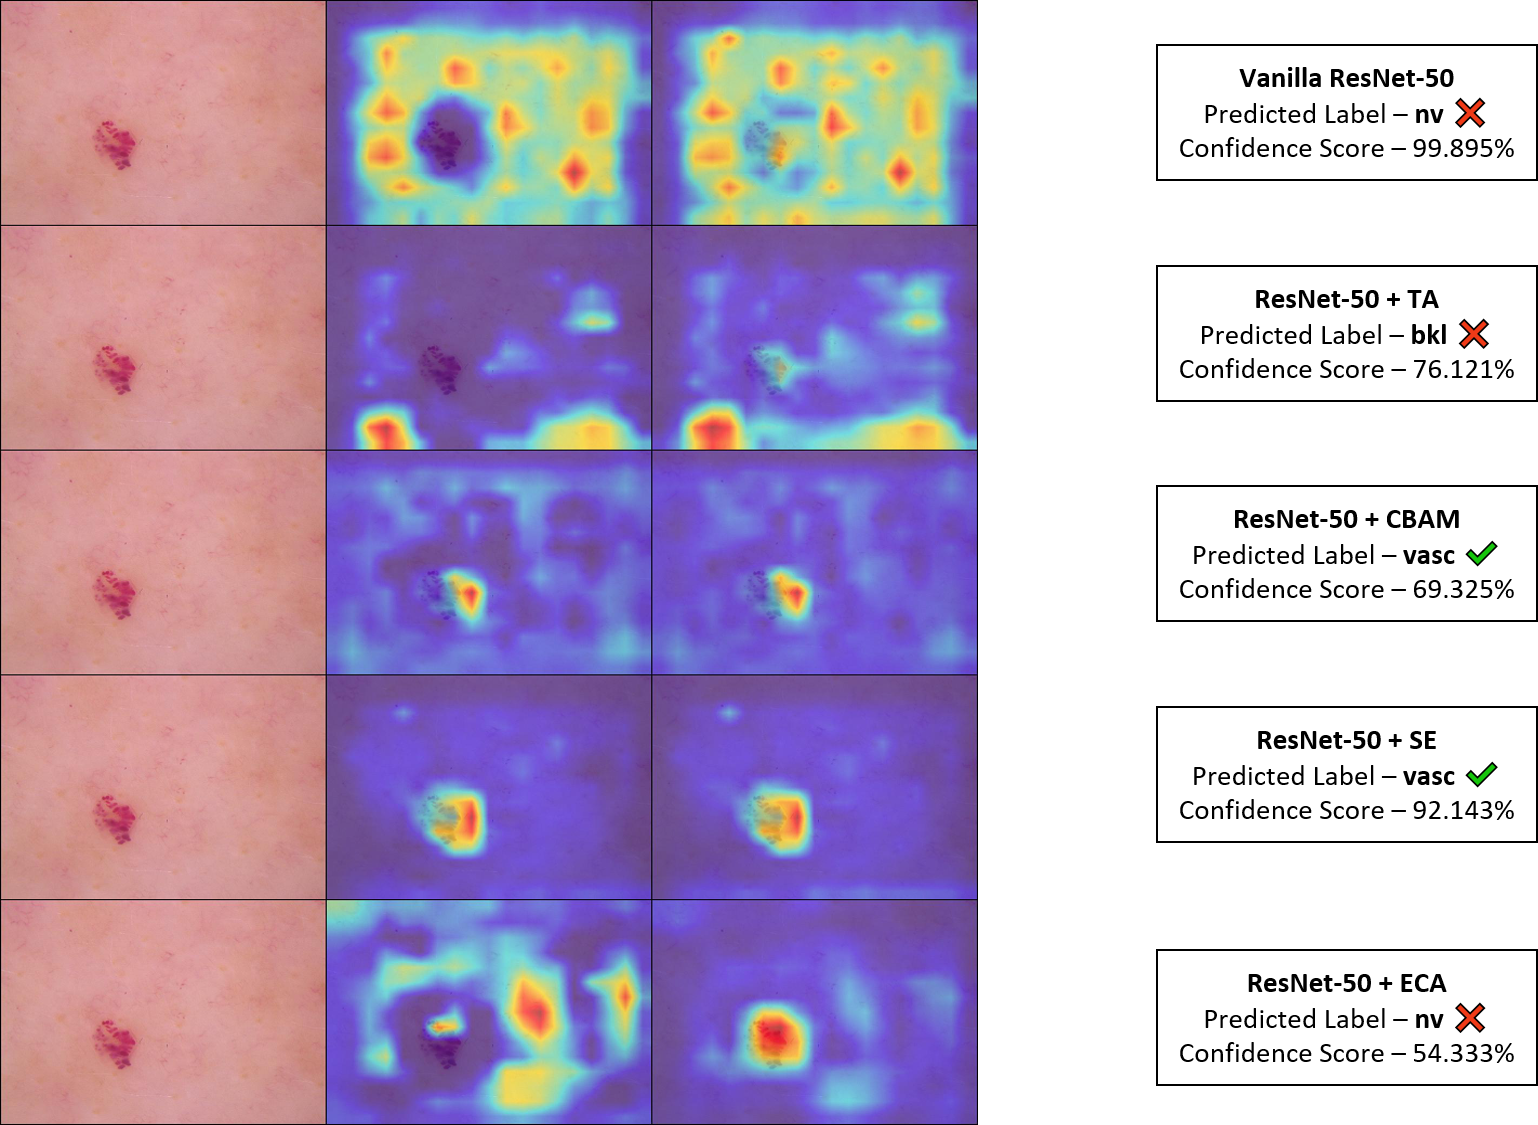}
\caption{Visualization of GradCAM and GradCAM++ respectively of the validation set in the VASC class.}
\label{fig:vasc}
\end{figure}
\end{appendices}
